# Supplementary material for: Photoassociative Spectroscopy of $^{87}$Sr
Source: arXiv:2011.11936 source file (2021-01-27)
Supplement: Supplementary file 1 [file SupplementaryMaterials_2021_01.pdf]

# 1 $^{84}\text{Sr}$ Lines

| $\nu$ | $E_\nu$<br>[GHz] | $\sigma$<br>[GHz] | $obs. - fit.$<br>[GHz] |
|-------|------------------|-------------------|------------------------|
| 76    | 7.31             | 0.03              | 0.03                   |
| 77    | 7.91             | 0.03              | 0.03                   |
| 78    | 8.52             | 0.03              | 0.00                   |
| 79    | 9.21             | 0.03              | 0.00                   |
| 80    | 9.91             | 0.03              | -0.04                  |
| 81    | 10.67            | 0.03              | -0.05                  |
| 82    | 11.52            | 0.03              | -0.03                  |
| 83    | 12.42            | 0.03              | -0.01                  |
| 86    | 15.40            | 0.03              | -0.02                  |
| 87    | 16.53            | 0.03              | -0.01                  |
| 89    | 18.88            | 0.03              | -0.10                  |
| 91    | 21.68            | 0.03              | -0.03                  |
| 93    | 24.73            | 0.03              | -0.04                  |
| 94    | 26.39            | 0.03              | -0.04                  |
| 95    | 28.10            | 0.03              | -0.08                  |
| 99    | 36.13            | 0.03              | -0.04                  |
| 100   | 38.38            | 0.02              | -0.06                  |
| 130   | 187.83           | 0.03              | 0.03                   |
| 131   | 196.71           | 0.03              | 0.02                   |
| 132   | 205.98           | 0.03              | 0.03                   |
| 133   | 215.73           | 0.07              | 0.18                   |

Table 1:  $^{84}\text{Sr}$  measured binding energies ( $E_\nu$ ), experimental uncertainties ( $\sigma$ ), and residuals ( $obs. - fit.$ ).

## 2 $^{86}\text{Sr}$ Lines

| $\nu$ | $E_\nu$<br>[GHz] | $\sigma$<br>[GHz] | $obs. - fit.$<br>[GHz] |
|-------|------------------|-------------------|------------------------|
| 77    | 7.83             | 0.02              | 0.08                   |
| 78    | 8.46             | 0.02              | 0.09                   |
| 82    | 11.31            | 0.03              | -0.01                  |
| 83    | 12.21            | 0.02              | 0.05                   |
| 88    | 17.35            | 0.02              | 0.06                   |
| 89    | 18.55            | 0.02              | 0.04                   |
| 94    | 25.73            | 0.02              | 0.02                   |
| 95    | 27.42            | 0.02              | 0.02                   |
| 100   | 37.32            | 0.03              | 0.02                   |
| 105   | 50.04            | 0.03              | 0.03                   |
| 109   | 62.58            | 0.03              | -0.03                  |
| 113   | 77.74            | 0.02              | -0.02                  |
| 118   | 100.83           | 0.03              | -0.04                  |
| 122   | 123.26           | 0.03              | 0.01                   |
| 127   | 156.96           | 0.03              | 0.06                   |
| 128   | 164.46           | 0.02              | -0.02                  |
| 131   | 189.01           | 0.03              | -0.03                  |
| 134   | 216.54           | 0.03              | -0.05                  |
| 136   | 236.80           | 0.03              | 0.04                   |

Table 2:  $^{86}\text{Sr}$  measured binding energies ( $E_\nu$ ), experimental uncertainties ( $\sigma$ ), and residuals ( $obs. - fit.$ ).

### 3 $^{87}\text{Sr}$ Lines

| $\nu$ | $E_\nu$<br>[GHz] | $\sigma$<br>[GHz] | $obs. - fit.$<br>[GHz] |
|-------|------------------|-------------------|------------------------|
| 76    | 6.67             | 0.11              | 0.11                   |
| 77    | 7.23             | 0.03              | 0.13                   |
| 78    | 7.79             | 0.03              | 0.11                   |
| 79    | 8.37             | 0.03              | 0.08                   |
| 80    | 9.05             | 0.03              | 0.11                   |
| 81    | 9.69             | 0.03              | 0.04                   |
| 82    | 10.42            | 0.11              | 0.04                   |
| 83    | 11.26            | 0.03              | 0.06                   |
| 84    | 12.09            | 0.03              | 0.06                   |
| 85    | 12.99            | 0.03              | 0.06                   |
| 86    | 13.95            | 0.05              | 0.06                   |
| 87    | 14.95            | 0.03              | 0.06                   |
| 88    | 16.02            | 0.03              | 0.07                   |
| 93    | 22.32            | 0.03              | 0.02                   |
| 95    | 25.36            | 0.03              | -0.02                  |
| 99    | 32.57            | 0.05              | -0.01                  |
| 100   | 34.55            | 0.04              | -0.06                  |
| 105   | 46.43            | 0.04              | -0.07                  |
| 108   | 55.05            | 0.04              | -0.08                  |
| 109   | 58.20            | 0.03              | -0.09                  |
| 110   | 61.49            | 0.06              | -0.12                  |
| 142   | 288.18           | 0.03              | -0.01                  |
| 143   | 300.67           | 0.03              | 0.01                   |
| 144   | 313.57           | 0.03              | -0.01                  |

Table 3:  $^{87}\text{Sr}$  measured binding energies ( $E_\nu$ ), experimental uncertainties ( $\sigma$ ), and residuals ( $obs. - fit.$ ).
